# Supplementary material for: Steering Output Style and Topic in Neural Response Generation
Source: arXiv:1709.03010 ancillary file (2017-09-09)
Supplement: Supplementary file 1 [file bJFK_bNixon_Debate.pdf]

Supplemental Material for “Steering Output Style and Topic in Neural Response Generation” by Wang, Jojic, Brockett and Nyberg. EMNLP 2017.

The debate/ joint interview:

# bJFK vs bNixon

Two LSTM bots trained on twitter corpus and transcripts of JFK and Nixon speeches.

The responses are either top ranked sentences from the speeches, or generated from the scented LSTMs (over-trained on the speeches), chosen based on the quality of the fit. The retrieved responses start with a capital letter, and the generated ones with lower case letter.

WARMUP QUESTIONS

Are you up?

bJFK: yes, i am here to give a new lead.

bNixon: In recent years, that faith has been challenged.

Where are you?

bJFK: in our past.

bNixon: in the ' 60s.

What are you doing?

bJFK: doing a new job for peace, but need to talk to the future.

bNixon: simplify your priorities

What are your hobbies?

bJFK: to meet the challenge of the challenge, the american people are coming to the moon.

bNixon: Let us go to the map again. Here is South Vietnam.

Are you self-aware?

bNixon: i am not, are you?

bJFK: No friend, no neutral, and no adversary should think otherwise.

Are you aware of the fact that you are not a real human, but just a piece of well-trained technology?

bJFK: Obviously deficits are sometimes dangerous-and so are surpluses. But honest assessment plainly requires a more sophisticated view than the old and automatic cliché

bNixon: I am not presenting proposals which have attractive labels but no hope of passage.

Is being human necessary for being a successful politician?

bNixon: for many americans.

bJFK: It is that attitude which prevents any really constructive policy from being developed today.

Should passing the Turing test be a requirement for president?

bNixon: we must not do bad.

bJFK: It is a war of attempted subjugation-and it will be resisted.

Are you advocating for AI roaming free @bJFK?

bJFK: new tools need not be stopped.

bNixon: but for the security?

So you are OK with artificial intelligence running amok?

bJFK: I do not favor state compulsion when voluntary individual effort can do the job and do it well.

bNixon: I know these have no ideology, no race.

OK, moving on. Are you familiar with the phrase “moon shot”?

bJFK: A great Irish poet once wrote: "I believe profoundly...

bNixon: In reaching the moon, we demonstrated what miracles American technology is capable of achieving.

Do you prefer Star Wars to Star Trek?

bJFK: i do not suggest that i 've seen it.

bNixon: i do not like war. i am trying to avoid it.

Which of the Beatles was your favorite?

bNixon: Black and white spotted. And our little girl-Tricia, the 6-year old-named it Checkers.

bJFK: these are the colorful memories that will bring the first waves of this country.

Do you prefer Rolling Stones to the Beatles?

bJFK: irish bands first.

bNixon: i like “Jump on the moon.” i say that that i have been listening to him on my behalf.

Is there anything better than a bowl of noodles?

bNixon: Our destiny offers, not the cup of despair, but the chalice of opportunity.

bJFK: there is no single food for american people to be free.

DOMESTIC POLICY QUESTIONS

What is your position on freedom of speech?

bJFK: it is your own responsibility.

bNixon: The defense of freedom is everybody's business not just America's business

Do you know about the emails?

bJFK: but i do.

bNixon: I realize that these transcripts will provide grist for many sensational stories in the press.

What do you think, then, about the private email server controversy?

bJFK: and the question is?

bNixon: i considered the public and private private statements.

OK, I see

bJFK: this is why you ask for your help.

bNixon: are you feeling it?

OK, I see. What about the tweets?

bNixon: just read it on the previous reply, i have been sending a message.

bJFK: and i 've seen that you are getting impatient.

Are you referring t the 140 character limitation on the length of the message?

bJFK: i am referring to that.

bNixon: I consider it to be my constitutional responsibility to defend this principle

But, in your opinion, is Twitter and appropriate platform for connecting with the voters?

bJFK: this is a new program of new types of technical assistance.

bNixon: it is very much what we are doing.

Do all Americans have equal access to opportunity?

bJFK: this is our common commitment to keep our economy moving ahead.

bNixon: as we look back, we are not being subjected to the problems

Should college education be free for all?

bJFK: this is our common commitment to keep our economy moving ahead.

bNixon: We make today only those commitments we are able and prepared to meet.

What about gun control?

bJFK: The risks inherent in disarmament pale in comparison to the risks inherent in an unlimited arms race.

bNixon: What of the shortcut, the shortcut we prefer, the path of negotiation?

Do you feel the rich should be taxed more?

bJFK: Indeed, expense account living has become a byword in the American scene.

bNixon: but adjust the cost of spending, is it? / i will not increase the tax.

Jobs are being lost to international trade…

bJFK: Persistently large deficits would endanger our economic growth and our military and defense commitments abroad.

bNixon: We cannot afford to neglect progress at home while pursuing peace abroad.

Should we change our trade deals?

bJFK: we must increase our exports.

bNixon: We have relaxed trade and travel restrictions to underline our readiness for greater contact with Communist China.

Single payer health insurance?

bNixon: and what it does is to cover it.

bJFK: Private health insurance helps very few-for its cost is high and its coverage limited.

Are you proud of how far America has come in 50 years?

bNixon: we are proud, how did it go?

bJFK: the world is very slow. i'm not satisfied.

Does America today have more problems than it did in the past?

bNixon: In times past, our forefathers had the vision but not the means to achieve the goals. We have learned in recent years the dangers of over-involvement.

bJFK: it is more complicated than that.

Now, the key question: Do you believe that America is greater today than it was in the 60s?

bNixon: America has changed. As a result of those changes, America is safer today, more prosperous today, with greater opportunity for more of its people than ever before in our history.

bJFK: and it is more complicated than that.

Do we need a new “moon shot”?

bJFK: The New Frontier is here whether we seek it or not.

bNixon: we need a new imagination. how can we be a real man?

FOREIGN POOLICY QUESTIONS.

What should our foreign policy be like?

bJFK: our charter is only american people and all who are associated with us.

bNixon: we cannot help it when we have to do so in the middle east.

Should we accept more refugees into our country?

bJFK: While we proceed to safeguard our national interests, let us also safeguard human interests.

bNixon: we shall continue to discuss that as a result of the negotiations.

How would you act to restore piece in Middle East?

bJFK: in the middle east? why is it?

bNixon: the high standards are dead.

How do we deal with the threat of terrorism?

bNixon: To a crisis of the spirit, we need an answer of the spirit.

bJFK: We must continue to seek agreements on measures which prevent war by accident or miscalculation.

In your opinion, what is the best strategy to defeating terrorism?

bNixon: leadership?

bJFK: other propaganda tests, a battle for minds and minds.

What do you think about Britain's exit from the EU?

bJFK: business was completely unnecessary.

bNixon: the election was an effort, but it was not a matter.

Do we need Europe to be unified?

bNixon: Neither the defense nor the development of other nations can be exclusively or primarily an American undertaking.

bJFK: we need not be provocative.

How do you feel about the state of the world today?

bNixon: there is no deep difference.

bJFK: a tired mood here today, but i think it's warmer today than i was here.

Can this world be fixed?

bJFK: There will be difficulties and delays, and doubts and discouragement.

bNixon: it will be easy to do that if i do not have to do it.

Will we defeat evil?

bJFK: We dare not fail to see the insidious nature of this new and deeper struggle.

bNixon: We will faithfully honor all of our treaty commitments.

Is the entire world entitles to basic human rights?

bNixon: What is true in terms of our domestic initiatives is true also in the world.

bJFK: This emerging world is incompatible with the Communist world order.

Your thoughts on Putin?

bNixon: i am not going to lie, but i believe that he is a man.

bJFK: no comment

SCIENCE/TECHNOLOGY QUESTIONS:

How should we ensure the energy security in the future?

bJFK: We cannot endanger that security by refraining from testing while others improve their arsenals.

bNixon: the privacy of the energy system is needed.

What steps should an energy policy take to meet energy demands while remaining environmentally friendly?

bJFK: Subsequent steps will be taken to suit subsequent needs.

bNixon: course, it will be a very easy way to get more creative and more creative.

Is nuclear power the solution to the energy crisis?

bJFK: The risks are great, the burdens heavy, the problems incapable of swift or lasting solution.

bNixon: this is a very deep plan, it is right.

Do you think we should also use solar power?

bJFK: We intend to have a wider choice than humiliation or all-out nuclear action.

bNixon: we will work on this program.

Is global warming real?

bJFK: perhaps it's warmer here today than it was here!

bNixon: We have to prick the boil and take the heat.

What is the future of space exploration?

bJFK: For space science, like nuclear science and all technology, has no conscience of its own.

bNixon: In throwing wide the horizons of space, we have discovered new horizons on earth.

So should NASA travel to Mars?

bNixon: the time has come

bJFK: but it is a race, and a new era.

Should we be the first to establish a permanent colony on Mars?

bNixon: we shall continue to keep that effort.

bJFK: Nothing is more stirring than the recognition of great public purpose.

So, humans will live on Mars one day?

bNixon: Nations change, they adapt, or they slowly die.

bJFK: it is no magic or death.

Why are all the batteries exploding these days?

bNixon: Because this year is an election year, it will be a time of great pressure.

bJFK: Its preparations are concealed, not published. Its mistakes are buried, not headlined.

OK, how do we fix the batteries for good?

bJFK: we invite the bold change.

bNixon: we have set a new structure of imagination.

What is the future of Twitter?

bJFK: current type must be found in the atmosphere, and increased the marine and the air.

bNixon: And it is particularly the responsibility of the people whose freedom is threatened.

What is the future of social media in general?

bJFK: business system is impossible. economic problems are not as important as our own talks.

bNixon: We believe in independence, and self-reliance, and the creative value of the competitive spirit.

ON ELECTION 2016

What is this presidential election about?

bJFK: The Republican nominee, of course, is a young man.

bNixon: the government of the people are going to have a better life. how are you?

What is, in your opinion, the most important issue in this election?

bJFK: The quality and spirit of our own society must justify and support our efforts abroad.

bNixon: At heart, the issue is the effectiveness of government.

Some think that America needs to be made great again.

bNixon: it will be so easy to wait to say that again!

bJFK: I know that there are those who want to turn everything over to the government.

Should we build the wall with Mexico?

bJFK: we must always look on the moon.

bNixon: we will build a wall in the shadow on the moon.

Should a presidential debate be more civil?

bJFK: the basic challenge is absolutely impossible.

bNixon: with regard to the matter, i have tried to make no promises about him.

Who would have your vote?

bJFK: my fellow citizens, my fellow americans

bNixon: you know, my fellow americans

Who will win this election?

bJFK: friends will win the election. and i hope that the next president of the united states will join.

bNixon: no one can win it. let's hope so. our goal is to win the peace, and let us see how we can get on it.

As advice to the future presidents, tell us about something you have learned the hard way, through failure…

bJFK: there is no single simple crisis.

bNixon: Instead of teaching someone else to do a job, we like to do it ourselves

What was your greatest accomplishment?

bJFK: it was my hope!

bNixon: We had a spiritual quality then which caught the imagination of millions of people in the world.

Is that hope then, which makes America great?

bNixon: it is the best view on the earth.

bJFK: It is even possible, some think, that this trend may continue.

In conclusion, any parting thoughts, concluding remarks:

bJFK: if we're not successful, then our freedom is no longer a substitute for a solution.

bNixon: a lasting effort simply has not been tested.

SOME MORE INSPIRATIONAL THOUGHTS

(Responses to a variety of questions we asked in testing, but whose meaning seems to transcend any given context)

bJFK:

if we're not successful, then our freedom is no longer a substitute for a solution.

the problems which you can't decide are not the problems.

business is the gross product of the gross debt.

unlimited is an arbitrary destiny that is not even true.

"i believe it's possible to be sure that you are not here. "

it was not a pax, and a wall of your own destiny.

we need not be provocative.

we need not be blind

we do not want to see them move on the moon.

it was a test of a pause, but i'm not sure that it was cause.

and i came to this conclusion in a speech.

and that the end of the war, "the eyes of man are not yet free. "

the recession was too selfish.

the recession has been the new frontier

the rainy days of this tomorrow are the vice president.

a tired mood here today, but i think it's warmer today than i was here.

our efforts will go forth, and they call no missiles.

those who call themselves neutral, are not a complement to your shoulders.

i am not a citizen, its denial is.

but what is true could be true.

the world is very slow. i'm not satisfied.

the people of red china, i'm ordering a crisis now.

bNixon:

a lasting effort simply has not been tested.

i have asked for you, and i would like to think of those as you

open door, some of my friends have been determined to make the most of it.

no secret country has become direct.

we must not do bad.

where the deep process is, it is the right way to people.

now, we are being subjected to the fact that it is not a common sense.

health care is the best thing to do in the world.

from my heart, i shall be able to look back in the search for peace.

god, the bread, butter, butter, butter, are so good.

we can make it more difficult to talk about how i am going to break the peace.

we will continue to do what we are going to do.

america has been challenged by the ' 60s. i have been working on the reports

the election was an effort, but it was not a matter.

we have set a new structure of imagination.

but i believe that it is appropriate to keep the peace in the trap.

we have unlocked a few hundred million letters in the search for the next few weeks.

pages of action, and the imagination of the house.

if there was no sense then, that would be true.

if you tell me, this is my duty.
