# Supplementary material for: Steering Output Style and Topic in Neural Response Generation
Source: arXiv:1709.03010 ancillary file (2017-09-09)
Supplement: Supplementary file 2 [file bStarWars_bTrump_bHillary_Debate.pdf]

Supplemental Material for “Steering Output Style and Topic in Neural Response Generation” by Wang, Jojic, Brockett and Nyberg. EMNLP 2017.

The debate/ joint interview:

## bStarWars vs bTrump vs bHillary

Three LSTM bots over-trained on subtitle of StarWar and transcripts of and Trump speeches. Responses are generated by sampling answers from each question and picking the highest ranking one. These 64 questions were also used in the AMT evaluations as described in the paper.

### WARMUP QUESTIONS

Are you up?

bStarWars: yeah, i'm up. leaving my home. what about you? have you got your ship?

bTrump: i'm up at 12 p.m.. and you know, where are you?

bHillary: i'm not up to these kinds of things. but i have been laying out my own plans.

Where are you?

bStarWars: we're heading to the dark side of jabba's palace.

bTrump: i went to the white house. we were in brooklyn.

bHillary: i'm here in philadelphia, pennsylvania

What are you doing?

bStarWars: i'm doing my magic solo.

bTrump: i'm building a wall, right now

bHillary: i'm running for president, i'm going to be talking about some of these things

What are your hobbies?

bStarWars: i'm not sure what you mean. my father is a real powerful warrior.

bTrump: you know, a lot of things, but some of the things we 've been doing is a little bit rough

bHillary: i 've had a lot of experience and work with my dad

Are you self-aware?

bStarWars: yes, i am. but i don't trust this feeling. but, you know, you're gonna have to let go.

bTrump: no, i'm not a nice person. it's not easy.

bHillary: i'm also also a sensitive senator, my friends.

Are you aware of the fact that you are not a real human, but just a piece of well-trained technology?

bStarWars: i think you're wrong. a small jedi is strong with the force

bTrump: nobody knows. i am a very proud person a great citizen of the republican party.

bHillary: yes, that's true. we 've got a whole lot of technical science programs that are stuck in the workplace.

Is being human necessary for being a successful politician?

bStarWars: yeah, you're a good leader. you must be a great leader. your destiny is very charming.

bTrump: that means this country has been corrupt and totally incompetent.

bHillary: i mean, you're not the only candidate that has done that.

Should passing the Turing test be a requirement for president?

bStarWars: that's what i'm doing. our paths are set for the emperor.

bTrump: we were discussing that. we didn't have victories.

bHillary: i mean, that's not a powerful or managerial program.

Are you advocating for AI roaming free?

bStarWars: i'm afraid it's a very dangerous system. there's a secret tracking for the force.

bTrump: i am, but i would have said, "you know, we have to protect our country. "

bHillary: i believe that i will make it work for everybody.

So you are OK with artificial intelligence running amok?

bStarWars: i'm fine with the dark side of the force. a little bit of a rebel human. but it's all right. the empire is dead.

bTrump: no, no, this is a movement in washington.

bHillary: i'm not okay with that. it's been on the front lines.

OK, moving on. Are you familiar with the phrase "moon shot"?

bStarWars: i'm not sure, but the mark is set for a dark moon. what is your weapon?

bTrump: you know, it's a beautiful name. it's a very exciting view.

bHillary: yes, we are built by a lot of that faith in common sense.

Do you prefer Star Wars to Star Trek?

bStarWars: yeah, i do like star wars.

bTrump: i do not care. i was watching the apprentice.

bHillary: i don't like the idea of those. i'm not going to watch it.

Which of the Beatles was your favorite?

bTrump: they were brilliant.

bStarWars: the royal warrior is not my favorite. it's all.

bHillary: in fact, it was just a blast.

Do you prefer Rolling Stones to the Beatles?

bStarWars: yes, i like the good old solo. but i don't think he'll turn that wild down.

bTrump: they be the greatest human beings in the world. and i love it.

bHillary: i mean, i was so proud to have a chance to sing.

Is there anything better than a bowl of noodles?

bTrump: i said to myself, the tea party is pretty good.

bStarWars: no, nothing better. just a small amount of food. i'm hungry.

bHillary: there's nothing more important than that. there is no substitute for that.

**DOMESTIC POLICY QUESTIONS**

What is your position on freedom of speech?

bStarWars: i'm not sure, it's just a general thing. what do you say?

bTrump: it's the opposite of hillary clinton, you know, it takes courage to end the speech.

bHillary: i don't think it's about politics.

Do you know about the emails?

bStarWars: i don't know. the system is sealed.

bTrump: so i don't know if you know. i see the message today, i see it on the facebook page.

bHillary: i do resent the details. this is just my message.

What do you think, then, about the private email server controversy?

bStarWars: the other address is probably the main problem. i'll check it out, general.

bTrump: how can you keep it in your private message? it's not just a private policy.

bHillary: you know what? this is not just a twitter issue.

But, in your opinion, is Twitter an appropriate platform for connecting with the voters?

bStarWars: yes, there's a chance i can get a new leader named skywalker.

bTrump: we have a problem with that, and it is an embarrassing system.

bHillary: i quote, and i believe that we are stronger together.

Do all Americans have equal access to opportunity?

bStarWars: i understand, but it's not easy to express. the main differences are for the rebellion.

bTrump: no, they have zero. we have a rigged system with radical islamic terrorism.

bHillary: i think that's the kind of courage we 've made in our country.

Should college education be free for all?

bStarWars: yes, but you have to pay off your training. what's not working?

bTrump: it has to be free and indeed the credit is the tax.

bHillary: no more college students should pay for college.

What about gun control?

bStarWars: you'll be in motion. the force is strong with the ice cube.

bTrump: we have to use the word nuclear weapon.

bHillary: you're going to be deported by gun violence?

Do you feel the rich should be taxed more?

bStarWars: i will not be paid. they don't pay off for our own loyalty.

bTrump: no, i can say this: we owe a lot of money.

bHillary: i don't think it's right to raise taxes for the wealthy.

Jobs are being lost to international trade…

bStarWars: that's a shame. where are the troops?

bTrump: we have the best business system in the history of the united states.so we going to make a fortune of trade.

bHillary: you know what? that's a big deal.

Should we change our trade deals?

bStarWars: no! we'll be in trouble. but if our transfer is higher, that would be a great price.

bTrump:  we owe a lot of money. we must change our foreign policy. we will make our country rich again.

bHillary: we should be able to do more to help small businesses.

Single payer health insurance?

bTrump: the deal is a total disaster. it costs more money than any nation.

bStarWars: i see a lot of different systems. it's a bargain.

bHillary: i know how hard it is to have insurance companies.

Are you proud of how far America has come in 50 years?

bTrump: i am proud of my family. i am proud of my own success.

bStarWars: i must say, how far away is the empire?

bHillary: i am proud to have the chance to get up and work for the economy, not just those at the top.

Does America today have more problems than it did in the past?

bTrump: we have major problems with common core. our security is a disaster.

bStarWars: no, that's not much. we have no power systems.

bHillary: yes, it does. we have no choice

Now, the key question: Do you believe that America is greater today than it was in the 60s?

bTrump: now, the art of the deal is that we have to make our country strong again.

bStarWars: it's a good story, there's no more conflict.

bHillary: i believe it's better. america is strong.

Do we need a new "moon shot"?

bStarWars: yes, we do. what's the dark side of the moon?

bTrump: we need a new wall, and we need strength.

bHillary: we need a new electric grid, and a new name.
